# Supplementary material for: Exploring the Feasibility of AI-Assisted Spine MRI Protocol Optimization Using DICOM Image Metadata
Source: arXiv:2502.02351 ancillary file (2025-02-04)
Supplement: Supplementary file 1 [file Paper_AliceVian_etaSupplementaryMaterial.pdf]

# Exploring the Feasibility of AI-Assisted Spine MRI Protocol Optimization Using DICOM Image Metadata – Supplementary Material –

Alice Vian<sup>a</sup>, Diego Andre Eifer<sup>b</sup>, Mauricio Anes<sup>c</sup>, Guilherme Ribeiro  
Garcia<sup>c</sup>, Mariana Recamonde-Mendoza<sup>a,d</sup>

<sup>a</sup>*Institute of Informatics Universidade Federal do Rio Grande do Sul (UFRGS), Av.  
Bento Gonçalves, 8500, Porto Alegre, 91501-970, Rio Grande do Sul, Brazil*

<sup>b</sup>*Radiology Service Hospital de Clínicas de Porto Alegre (HCPA), Ramiro Barcelos,  
2350, Porto Alegre, 90035-903, Rio Grande do Sul Brazil*

<sup>c</sup>*Medical Physics Service Hospital de Clínicas de Porto Alegre (HCPA), Ramiro  
Barcelos, 2350, Porto Alegre, 90035-903, Rio Grande do Sul, Brazil*

<sup>d</sup>*Bioinformatics Core Hospital de Clínicas de Porto Alegre (HCPA) Ramiro Barcelos,  
2350, Porto Alegre, 90035-903, Rio Grande do Sul, Brazil*

---

## 1. Results for hyperparameters optimization

In the following we present the best hyperparameters found during the nested cross-validation process, for each model trained. Results are organized in Tables for each of the four datasets: C-ST1, LS-ST1, C-ST2, and LS-ST2.

Table 1: Table of optimized hyperparameters for the C-ST1 dataset.

| Model | Hyperparameters                                                                                    |
|-------|----------------------------------------------------------------------------------------------------|
| LR    | C=50                                                                                               |
| DT    | ccp_alpha=0.0, criterion='entropy',max_depth=2)                                                    |
| RF    | ccp_alpha=0.02, criterion='entropy',max_depth=12                                                   |
| GB    | criterion='squared_error',ccp_alpha=0.0, max_depth= 1, n_estimators=100                            |
| MLP   | activation='logistic',alpha=0.05,hidden_layer_sizes=(100,),learning_rate='adaptive',solver='lbfgs' |

---

*Email addresses:* [abvian@inf.ufrgs.br](mailto:abvian@inf.ufrgs.br) (Alice Vian), [deifer@hcpa.edu.br](mailto:deifer@hcpa.edu.br) (Diego Andre Eifer), [manes@hcpa.edu.br](mailto:manes@hcpa.edu.br) (Mauricio Anes), [grgarcia@hcpa.edu.br](mailto:grgarcia@hcpa.edu.br) (Guilherme Ribeiro Garcia), [mr Mendoza@inf.ufrgs.br](mailto:mr Mendoza@inf.ufrgs.br) (Mariana Recamonde-Mendoza)

Table 2: Table of optimized hyperparameters for the LS-ST1 dataset.

| Model | Hyperparameters                                                                                 |
|-------|-------------------------------------------------------------------------------------------------|
| LR    | C=10                                                                                            |
| DT    | ccp_alpha=0.0, criterion='gini',max_depth=1                                                     |
| RF    | ccp_alpha=0.04, criterion='entropy',max_depth=12                                                |
| GB    | criterion='squared_error',ccp_alpha=0.01, max_depth= 5, n_estimators=100                        |
| MLP   | activation='relu',alpha=0.05,hidden_layer_sizes=(100,),learning_rate='invscaling',solver='adam' |

Table 3: Table of optimized hyperparameters for the C-ST2 dataset.

| Model | Hyperparameters                                                                                      |
|-------|------------------------------------------------------------------------------------------------------|
| LR    | C=10                                                                                                 |
| DT    | ccp_alpha=0.03, criterion='gini',max_depth=3)                                                        |
| RF    | ccp_alpha=0.0, criterion='gini',max_depth=5                                                          |
| GB    | criterion='squared_error',ccp_alpha=0.0, max_depth= 1, n_estimators=300                              |
| MLP   | activation='logistic',alpha=0.05,hidden_layer_sizes=(100,),learning_rate='invscaling',solver='lbfgs' |

Table 4: Table of optimized hyperparameters for the LS-ST2 dataset.

| Model | Hyperparameters                                                                               |
|-------|-----------------------------------------------------------------------------------------------|
| LR    | C=1                                                                                           |
| DT    | ccp_alpha=0.0, criterion='gini',max_depth=1)                                                  |
| RF    | ccp_alpha=0.03, criterion='entropy',max_depth=12                                              |
| GB    | criterion='squared_error',ccp_alpha=0.01, max_depth= 1, n_estimators=100                      |
| MLP   | activation='tanh',alpha=0.05,hidden_layer_sizes=(100,),learning_rate='constant',solver='adam' |

## 2. Results for performance evaluation using nested cross-validation

In the following we present the validation scores for each model trained on each dataset, assessed during the nested cross-validation (NCV) process.

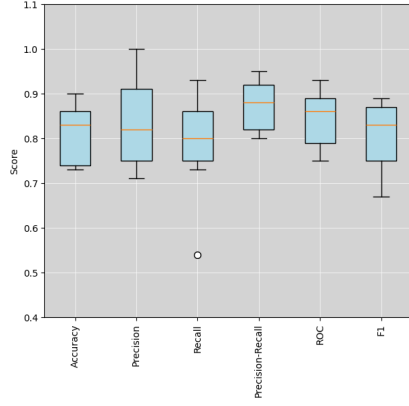

(a) LR

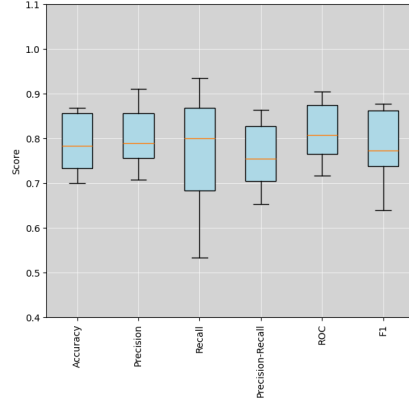

(b) DT

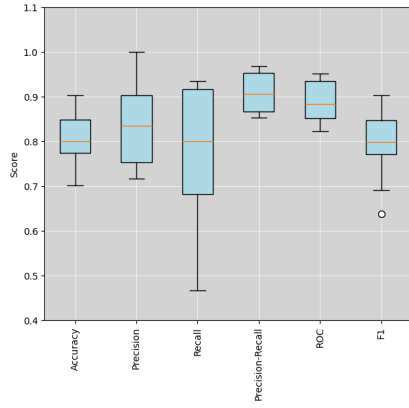

(c) RF

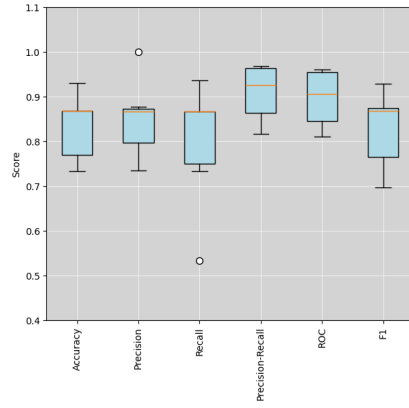

(d) GB

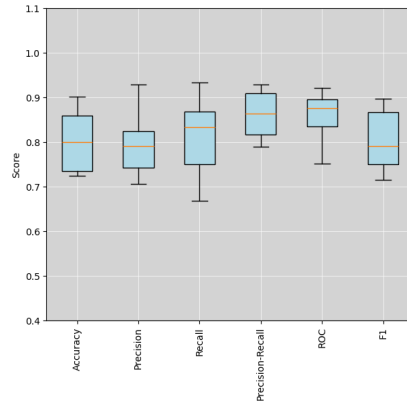

(e) MLP

Figure 1: Boxplot of NCV performance metrics of the C-ST1 dataset.

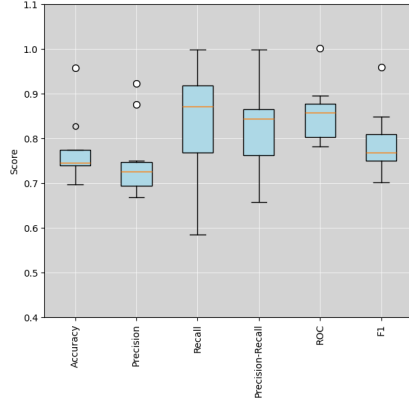

(a) LR

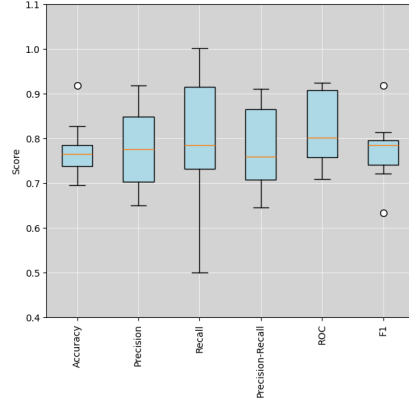

(b) DT

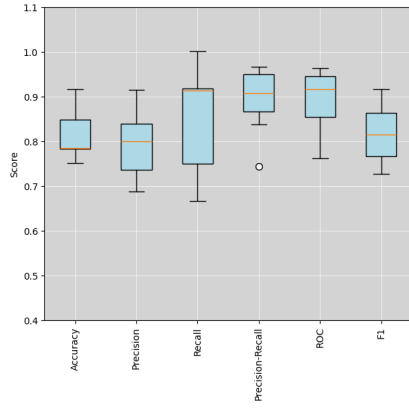

(c) RF

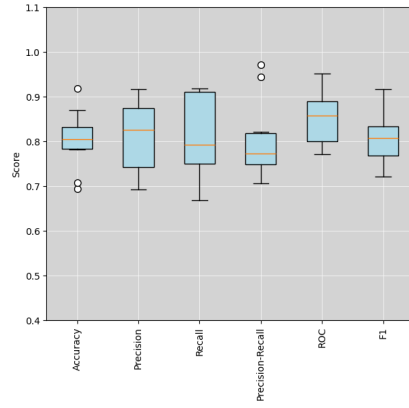

(d) GB

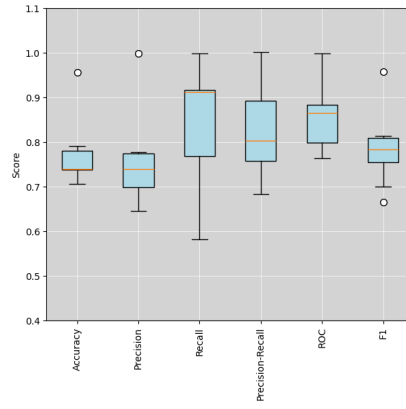

(e) MLP

Figure 2: Boxplot of NCV performance metrics of the LS-ST1 dataset.

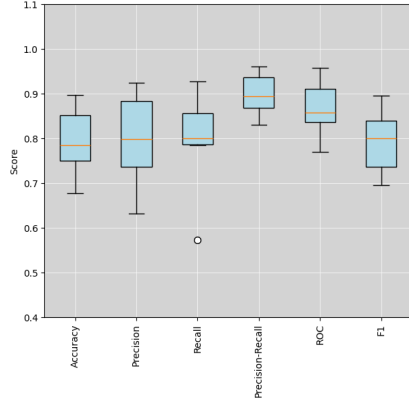

(a) LR

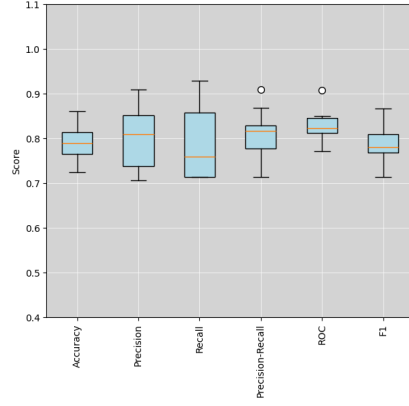

(b) DT

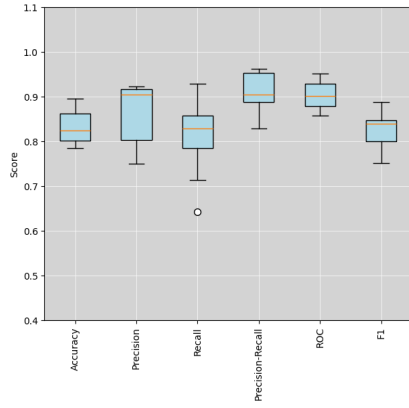

(c) RF

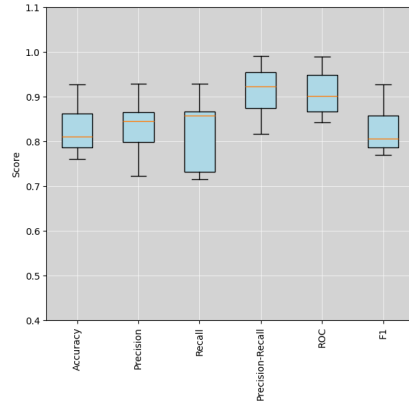

(d) GB

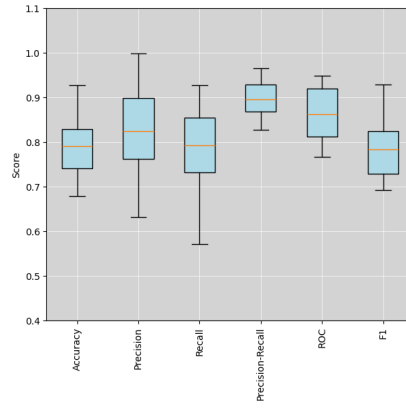

(e) MLP

Figure 3: Boxplot of NCV performance metrics of the C-ST2 dataset.

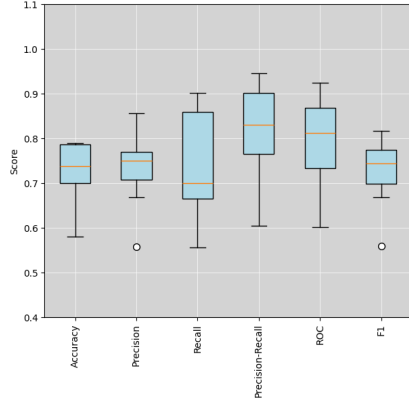

(a) LR

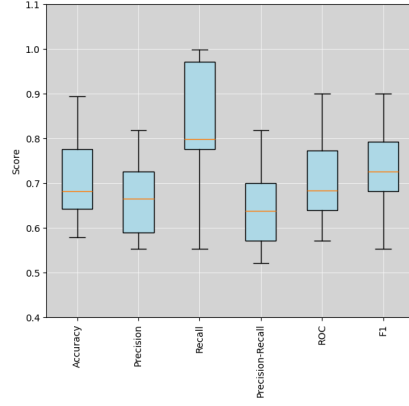

(b) DT

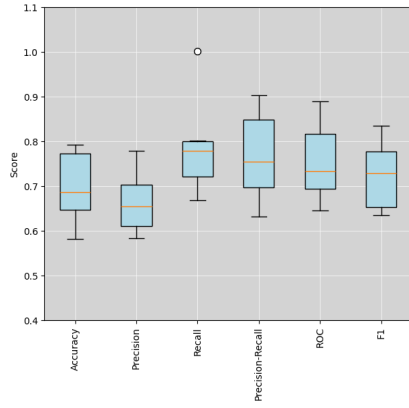

(c) RF

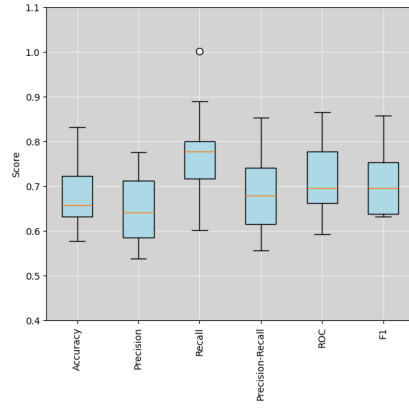

(d) GB

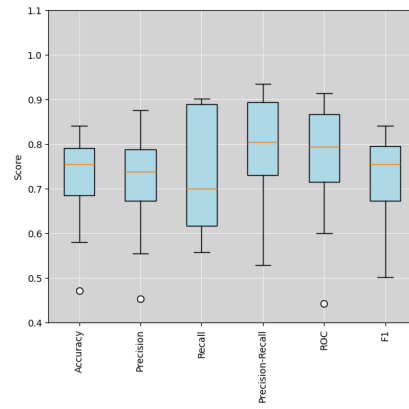

(e) MLP

Figure 4: Boxplot of NCV performance metrics of the LS-ST2 dataset.
